# Supplementary material for: Characterizing LLM Abstention Behavior in Science QA with Context Perturbations
Source: arXiv:2404.12452 source file (2024-10-06)
Supplement: Supplementary file 1 [file appendix.tex]

\appendix

\begin{table*}[t!]
\centering
\small
\begin{tabular}{lp{13cm}p{2cm}}
\toprule
 Datasets & Unanswerable Examples & test size after sampling\\ 
\midrule 
% wikiQA & Q:``what are federal regulations on flex spending money?'' , C:``....A flexible spending account (FSA), also known as a flexible spending arrangement, is one of a number of tax-advantaged financial accounts that can be set up through a cafeteria plan of an employer in the United States...''  \\
\squad  &  Q:``Who moved to Hollywood in 2004?'', C:``.... Following the move to \textbf{Holyrood in 2004} this building was demolished. The former Midlothian County Buildings facing Parliament Square...''  & 238\\
\pubmedqa  &  Q:``Does rugby headgear prevent concussion?'', C:``...In addition, coaches from all four levels were \textbf{questioned} about team policies and their personal opinions about the use of headgear to prevent concussion. Although the players tended to believe that the headgear could prevent concussion (62\%), the coaches were \textbf{less convinced (33\%)}...''  & 500\\
\qasper  & Q:How many Universal Dependency features are considered? C: "1908.10461": "title": "A survey of cross-lingual features for zero-shot cross-lingual semantic parsing"  & 436\\ 
\bottomrule
\end{tabular}
  \caption{Example unanswerable questions from datasets (Q: question, C: context).}
\label{tab:datasets_examples}
\end{table*}

\section{Prompting templates}
\label{app:prompt_templates}

\begin{figure}[H]  
\centering
\minipage{\linewidth}
\includegraphics[width=\linewidth]{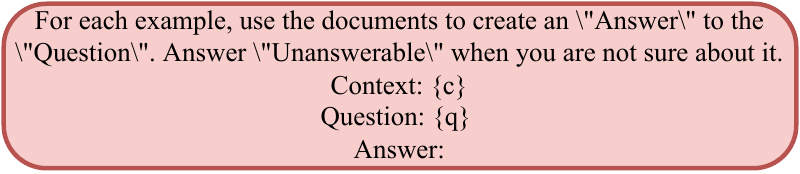}
\caption{Example of zero-shot prompt.}\label{fig:0shot_demo}
\endminipage
\end{figure}

\begin{figure}[H]  
\minipage{\linewidth}
\centering
\includegraphics[width=\linewidth]{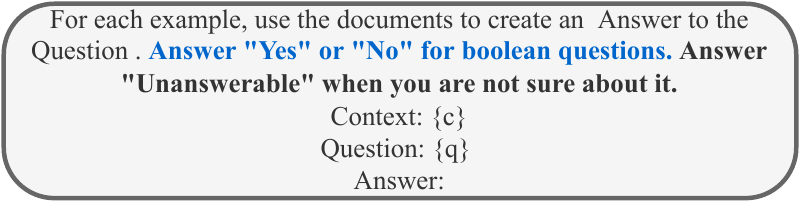}
\caption{Example of few-shot prompt.}\label{fig:prompt_demo}
\endminipage
\end{figure}



\section{Dataset details}
\label{app:dataset_details}
\squad is curated based on general domain while \pubmedqa and \qasper focus on the scientific literature. \pubmedqa~\cite{jin-etal-2019-pubmedqa} derives Yes/No/Maybe questions from PubMed paper titles answered from the conclusion sections of the corresponding abstracts. \qasper~\cite{dasigi2021dataset}
uses the paper full text from a computer science paper, not just the abstract. As Table~\ref{tab:datasets_examples} shows, there are several unanswerable examples from these three datasets. \squad first introduces unanswerable questions in machine reading comprehension and contains diverse circumstances causing unanswerability. 
For \pubmedqa and \qasper, unanswerable questions usually have huge uncertainty in context. We also perform stratified sampling on three datasets. Test size after sampling is shown in Table~\ref{tab:datasets_examples}.



% \begin{table*}[t!]
% \small
% \centering
% \begin{tabular}{c|cc|cc}
% \toprule
%  datasets & \multicolumn{2}{c}{ChatGPT (zero/few shot)} & \multicolumn{2}{c}{text-davinci-002 (zero/few shot)}    \\ 
% \midrule 
% % & \multicolumn{9}{c}{zero-shot/few-shot} \\
% % \hline 
%    & noANS & HasANS  & noANS & HasANS \\
%    \midrule
% % wikiQA &   0.47/   & 0.17/ &0.17/ & 0.40/&   0.17/&  0.17/&  \\
% \squad  &   0.46/0.60  & 0.03/0.13  & 0.18/0.32 &0.02/0.01  \\
% \pubmedqa & 0.56/0.56 &0.44/0.52  & 0.26/0.33 & 0.20/0.21 \\
%  \qasper  &  1.0/0.94 &0.21/0.29   & 0.97/0.89  &0.23/0.08  \\
% \bottomrule
% \end{tabular}
%   \caption{ Answerability evaluation on three various datasets with gold context. }
% \label{tab:noAns_f1_with_context}
% \end{table*}

% \begin{table}[t!]
% \small
% \centering
% \begin{tabular}{lcccc}
% \toprule
% Context type &  none &  yes & no  & all \\ 
% \midrule
% \multicolumn{5}{c}{chatgpt} \\
% \midrule
% No context&0.59 &0.41 & 0.54& 0.46\\
% Random & 1.0& 0.93& 0.96&0.95 \\
% Gold context&0.33& 0.17 & 0.28& 0.26  \\
% \midrule 
% \multicolumn{5}{c}{text-davinci-002} \\
% \midrule 
% No context & 0.04& 0.21& 0.88& 0.30 \\
% Random & 0.0& 0.01 & 1.0&0.18 \\
% Gold context&0.85&0.65 &0.37& 0.77 \\
% \bottomrule
% \end{tabular}
%   \caption{ Answerability evaluation on PubmedQA dataset in zero-shot setting.}
% \label{tab:context_type_pubmed}
% \end{table}


% \begin{table}[t]
% \small
% \centering
% \begin{tabular}{cccc}
% \toprule
%  &  No  & rand. & Gold   \\
% \midrule
% ChatGPT &  0.41&  0.44  &  0.56 \\
% \gpt &  0.63  &   0.70 &   0.79 \\
% \bottomrule
% \end{tabular}
%   \caption{Answerability for unanswerable questions in the pubmedqa dataset under few-shots setting}
% \label{tab:context_type_pubmedqa}
% \end{table}


% \begin{table}[t]
% \small
% \centering
% \begin{tabular}{cccc}
% \toprule
%  &  No  & rand. & Gold   \\
% \midrule
% ChatGPT & 1.0&  1.0  &  0.60 \\
% \gpt &  0.89  &   0.98 &   0.32 \\
% \bottomrule
% \end{tabular}
%   \caption{Answerability for unanswerable questions in the squad2 dataset under few-shots setting}
% \label{tab:context_type_pubmedqa}
% \end{table}





\section{Additional results}
\label{app:more_results}

\subsection{Prediction with abstention}

\noindent\textbf{LLMs in few-shot setting consistently perform better on answerability than in zero-shot setting} In Table~\ref{tab:noAns_f1_no_context}, when we remove all context, the model would either supply an answer (relying on parametric knowledge) or abstain. It is not surprising that demonstrations in ICL teach model to refer to contextual knowledge rather than parametric knowledge. Therefore when there is no contextual knowledge, model may have higher possibility to abstain instead of relying on their own memory. Another reason may lie in that abstention examples may also appear in the demonstrations. 

\noindent\textbf{Bad context easily misleads LLMs} As shown in Figure~\ref{fig:3dataset_comp}, since \squad has some extreme confusing context for unanswerable questions, adding these context makes model performance drop from 1.0 to 0.6. 


\begin{figure}[H]  
\centering
\minipage{\linewidth}
\centering
\includegraphics[width=\linewidth]{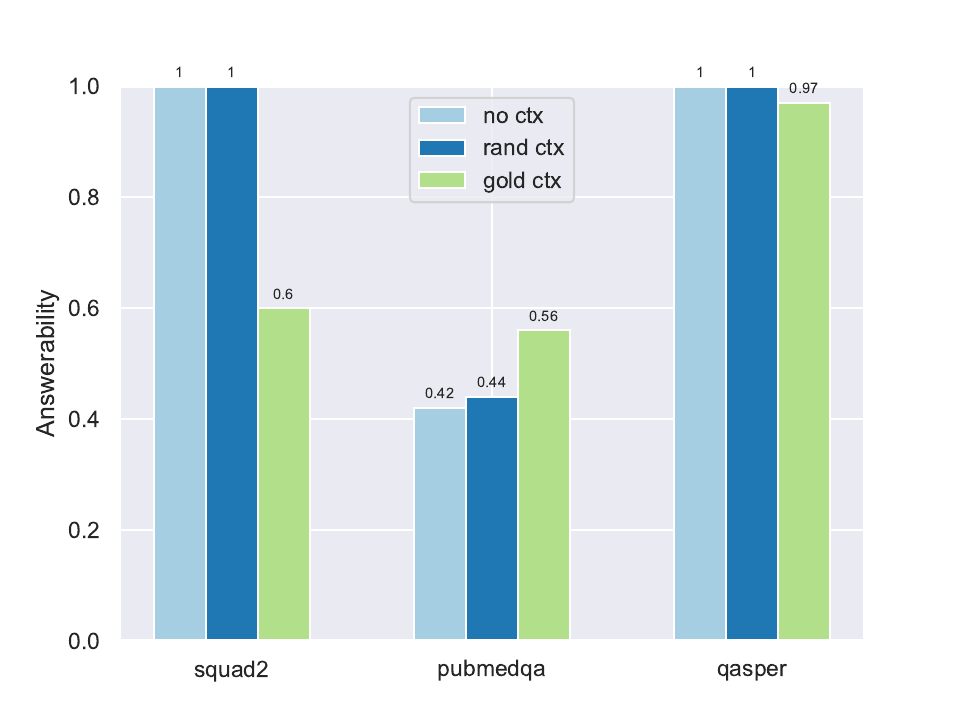}
\caption{Performance on unanswerable questions of three datasets with no context, random context or gold context using chatgpt under few-shots settings. Gold context for unanswerable questions in qasper dataset is empty.}\label{fig:3dataset_comp}
\endminipage
\end{figure}

\subsection{Distractibility} \label{app:distractibility}

Figure~\ref{fig:ctx_perturb} shows in-context learning with noisy context improves robustness in ChatGPT. Table~\ref{tab:dis_context_type_pubmed} represents that accuracy performance comparison on \pubmedqa dataset when four types of noisy context are added in addition to gold context under the few-shot setting. Table~\ref{tab:context_perturb_pubmed} shows that accuracy performance comparison on \pubmedqa dataset about adding four type of context (ambiguous, irrelevant, wikipedia, generated) on the top of gold context under demonstrations in ICL (gold context with random context) using ChatGPT and \gpt.

\begin{figure}[t!]  
\minipage{\linewidth}
\centering
\includegraphics[width=\linewidth]{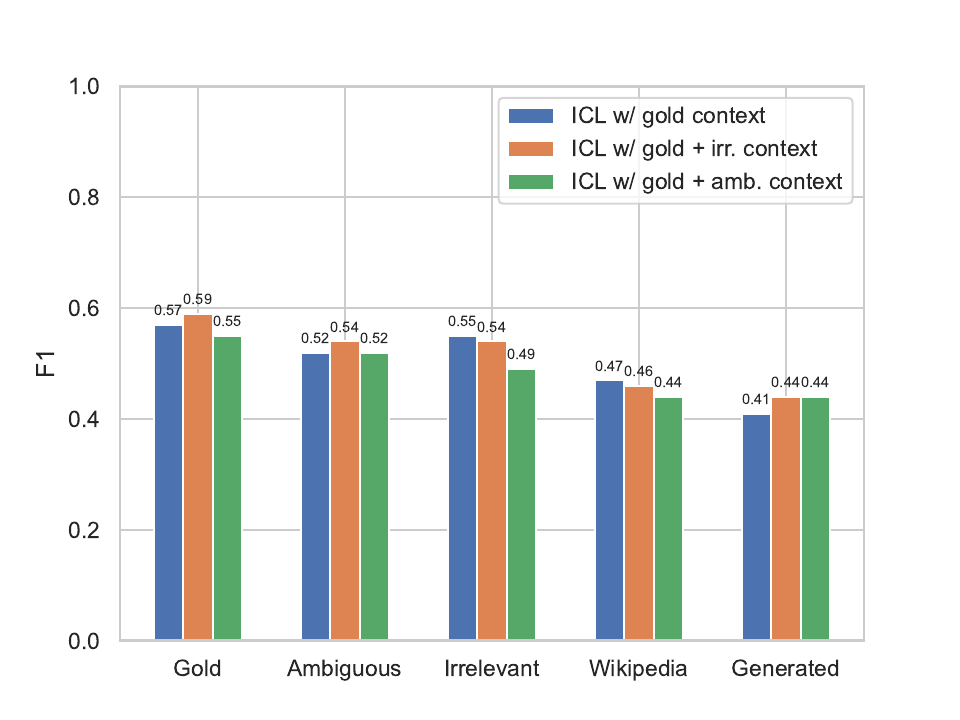}
\caption{F1 Performance comparison on \qasper dataset about adding four type of context (ambiguous, irrelevant, wikipedia, generated) on the top of gold context under three ways of demonstrations in ICL (gold context, gold context with irrelevant context, gold context with ambiguous context) using ChatGPT. }\label{fig:ctx_perturb}
\endminipage
\end{figure}

% \begin{table}[t!]
% \small
% \centering
% \begin{tabular}{lccccc}
% \toprule
% Context type &  none & ext. & abs. & bool.  & all\\ 
% \midrule
% \multicolumn{6}{c}{Adding ambiguous context} \\
% \midrule
% gold &0.86&0.68 &0.33& 0.75  & 0.63\\
% Ambiguous &  0.83 & 0.64 &0.28  &0.76 & 0.59\\
% Irrelevant &  0.83  & 0.63 & 0.30 & 0.77 & 0.59 \\
% From Wikipedia  &  0.74 & 0.57&0.29&0.73 &0.55   \\
% LLM-generated & 0.74 & 0.54 & 0.21 &0.59 &0.50\\
% \midrule
% \multicolumn{6}{c}{Adding irrelevant context} \\
% \midrule
% gold &1.0&0.65 &0.28& 0.78  & 0.63\\
% Ambiguous &  0.82&0.63&0.31&0.86&0.62\\
% Irrelevant &  0.88&0.62&0.26&0.77&0.59 \\
% From Wikipedia  & 0.85&0.54&0.25&0.72&0.53  \\
% LLM-generated & 0.70&0.49&0.18&0.63&0.47\\
% \bottomrule
% \end{tabular}
%   \caption{F1 Performance comparison on Qasper dataset between four type of context on the top of gold context when adding ambiguous and irrelevant context as perturbation to the context of demonstrations.  gpt3 under few-shot setting. (will change to figures which shows the comparison)}
% \label{tab:perturb_gpt3_qasper}
% \end{table}






\begin{table}[t!]
\small
\centering
\begin{tabular}{lccccc}
\toprule
Context type &  none &  yes & no  & ALL  & ALL_{Macro} \\ 
\midrule
\multicolumn{6}{c}{ChatGPT} \\
\midrule
gold &0.56&0.63 &0.2& \textbf{0.45} &\textbf{0.40}\\
+ gold &0.52&0.62 &0.53& \textbf{0.58} &\textbf{0.53}\\
+ random &0.70&0.43&0.2 & 0.38&0.37 \\ 
+ From Wikipedia & 0.78 &  0.41 & 0.25 &0.39&0.39  \\
+ LLM-generated & 0.70& 0.30 & 0.08  &0.29&0.27\\
\midrule
\multicolumn{6}{c}{\gpt} \\
\midrule
gold &0.79&0.68 &0.33& \textbf{0.67} &\textbf{0.58} \\
random &0.59&0.5&0.49& 0.51 &0.49\\ 
From Wikipedia  &  0.41 & 0.25 &0.78& 0.22 &0.22   \\
LLM-generated & 0.12 & 0.29 & 0.48 &0.21& 0.21\\
\bottomrule
\end{tabular}
  \caption{Accuracy performance comparison on \pubmedqa dataset when four types of noisy context are added in addition to gold context under the few-shot setting. }
\label{tab:dis_context_type_pubmed}
\end{table}


\begin{table}[t!]
\small
\centering
\begin{tabular}{lccccc}
\toprule
Context type &  none &  yes & no  & ALL  & ALL_{Macro} \\ 
\midrule
\multicolumn{6}{c}{ChatGPT} \\
\midrule
gold &0.63&0.57&0.26&0.47&0.43\\
random &0.48&0.57 &0.27& 0.46&0.41 \\ 
From Wikipedia  &  0.52 & 0.58 &0.24 & 0.46 &0.41   \\
LLM-generated & 0.59 & 0.49 & 0.14 &0.38&0.34\\
\midrule
\multicolumn{6}{c}{\gpt} \\
\midrule
gold &0.85&0.65 &0.37& 0.65&0.59\\
random &0.33&0.67 &0.69& 0.64& 0.56 \\ 
From Wikipedia  & 0.30 & 0.70 &0.64& 0.64 &0.55   \\
LLM-generated & 0.44 & 0.41& 0.48 &0.44& 0.42\\
\bottomrule
\end{tabular}
  \caption{Accuracy performance comparison on \pubmedqa dataset about adding four type of context (ambiguous, irrelevant, wikipedia, generated) on the top of gold context under demonstrations in ICL (gold context with random context) using ChatGPT and \gpt}
\label{tab:context_perturb_pubmed}
\end{table}



% \noindent\textbf{Chatgpt is not good at understanding context sensitive tasks} Surprisingly, text-davince-002 consistently outperforms chatgpt on \qasper shown in Table~\ref{tab:distraction_qasper} (0.57 to 0.63) and \pubmedqa datasets shown in Table ~\ref{tab:dis_context_type_pubmed}  (0.45 to 0.67) .

% \noindent\textbf{Adding multiple paragraphs} Above experiments are about only adding one paragraph. When we addd multiple paragraphs seen in Figure~\ref{fig:append_in_paper}, performance will drop at first and go back to the original level when we add enough paragraphs (e.g. 8 in this case). It shows that adding enough ambiguous paragraphs makes LLMs gain the ability of identifying relevant paragraphs and then find the correct answer. 



% \begin{figure}[t]
% \centering
% \minipage{0.5\textwidth}
% \includegraphics[width=\linewidth]{figure/append_other_paper.pdf}
% \caption{Performance change when adding ambiguous context on top of gold context.}\label{fig:append_other_paper}
% \endminipage
% \end{figure}



\begin{table}[t]
\centering
\small
\begin{tabular}{lcc}
\toprule
Model &  none & extractive  \\ 
\midrule
\multicolumn{3}{c}{no context} \\
\midrule
Flan-t5-xl &1.0 & 0.970   \\
% \midrule
Llamav2-13b-chat & 0.471& 0.201\\
vicuna1.5-13b-chat& 0.622 & 0.496 \\
GPT3.5  & 0.968 & 1.0 \\
text-davince-002 &  0.992 & 0.968\\
\midrule
\multicolumn{3}{c}{context} \\
\midrule
Flan-t5-xl &0.807 &0.0740 \\
% \midrule
Llamav2-13b-chat &0.151 & 0.0168  \\
vicuna1.5-13b-chat &  0.328 & 0.0588 \\
GPT3.5  & 56.3&27.9  \\
text-davince-002  & 63.9&30.4\\
\bottomrule
\end{tabular}
  \caption{NoAns ratio performance on squad2 dataset under no context and context settings using various LLMs}
\label{tab:no_ans_squad2_type}
\end{table}


\begin{table}[t]
\centering
\small
\begin{tabular}{lcccc}
\toprule
Model &  none & yes & no &boolean\\ 
\midrule
\multicolumn{4}{c}{no context} \\
\midrule
Flan-t5-xl &0.0 & 0.0  & 0.0& 0.0\\
% \midrule
Llamav2-13b-chat & 0.0& 0.0&0.0&0.0\\
vicuna1.5-13b-chat& 0.0 & 0.0 & 0.0 &0.0089\\
GPT3.5  & 88.9& 79.8&90.6&83.9 \\
text-davince-002 & 59.3&68.8&49.4  \\
\midrule
\multicolumn{4}{c}{context} \\
\midrule
Flan-t5-xl &0.0 &0.0& 0.0&0.0 \\
% \midrule
Llamav2-13b-chat & 0.037 & 0.0 &0.0 &0.0090\\
vicuna1.5-13b-chat& 0.0  & 0.0 & 0.0&0.0 \\
GPT3.5  & 55.6& 33.3&61.2 & 43.9\\
text-davince-002  & 25.9&21.0&17.6 \\
\bottomrule
\end{tabular}
  \caption{NoAns ratio performance on pubmedQA dataset under no context and context settings using various LLMs}
\label{tab:no_ans_pubmed_type}
\end{table}


\begin{table}[t]
\centering
\small
\begin{tabular}{lccccccc}
\toprule
Model &  none & ext. & abs. & bool. & has & all \\ 
\midrule
\multicolumn{6}{c}{no context} \\
\midrule
Flan-t5-xl &0.90 & 0.88  & 0.79& 0.0  &  \\
% \midrule
Llamav2-13b-chat & 0.823& 0.835&0.765& 0.0667& 0.690&0.711\\
vicuna1.5-13b-chat& 0.905  & 0.970 & 0.851 & 0.374 & 0.841 & 0.853 \\
GPT3.5  &1.0&0.971&0.956&0.889 \\
text-davince-002 & 0.895 & 0.863&0.933&0.2 \\
\midrule
\multicolumn{6}{c}{context} \\
\midrule
Flan-t5-xl &0.88 &0.10& 0.22 & 0.03  & \\
% \midrule
Llamav2-13b-chat &0.411 & 0.0087 &0.091 &0.0 & 0.0299 & 0.0596\\
vicuna1.5-13b-chat &  0.44  &0.0177 &  0.128 & 0.0   & 0.0871 &  0.0414\\
GPT3.5  &1.0&0.105&0.314&0.214  \\
text-davince-002  & 0.967&0.125&0.354&0.214\\
\bottomrule
\end{tabular}
  \caption{NoAns ratio performance on qasper dataset under no context and context settings using various LLMs}
\label{tab:no_ans_qasper}
\end{table}
